# Supplementary material for: Invariant measures for interval maps without Lyapunov exponents
Source: arXiv:2102.06795 source file (2021-02-22)
Supplement: Supplementary file 1 [file Appendix.tex]

\section{Appendix}

In this appendix we will study the natural extension of the map $f$ given by Theorem \ref{thm:1}. The ideas presented 
here are classical and, since the work of Ledrappier, see \cite{Led81}, they had been used to apply the Pesin theory to
to interval maps, see \cite{Led81} in the smooth case, and \cite{Dob14}, \cite{Dob15}, \cite{Lim18}, and references 
therein for the case of interval maps with critical points and discontinuities. In particular, we will be 
interested in the backward Lyapunov
exponent (see definition below), since it is needed in the construction of the Pesin coordinate. These systems of
coordinates are a key tool in Pesin theory, and they give a uniform hyperbolic linearization of the original system.
Lemma \ref{lem:back_lyap_exp} below, tell us that we cannot rule out the possibility of constructing Pesin coordinates for the map $f$.

For the map $f \colon I \longrightarrow I$, let \[\hI \= \{ \overline{x} = \ldots x_{-1}:x_0x_1 \ldots 
\in I^{\Z} \colon  f(x_{n-1}) = x_n \}.  \] Endow $\hI$ with the distance 
\[ \hat{d}(\overline{x}, \overline{y}) \= \sup \{2^n|x_n - y_n| \colon n\leq 0 \}.  \] Then
$(\hI,\hat{d})$ is a compact metric space. 

For each $n \in \Z$ define 
\begin{align*}
  \pi_n \colon \hI &\longrightarrow I\\
  \overline{x} &\mapsto \pi_n(\overline{x}) =x_n.
\end{align*}
So $\pi_n$ is the projection into the $n$th coordinate. Let $\hat{cB}$ be the $\sigma-$algebra in 
$\hI$ generated by $\{ \pi_n \colon n \leq 0 \}$. The natural extension of $f$ is the map 
\[ \overline{f} \colon \hI \longrightarrow \hI, \] defined by \[ \overline{f}(\ldots x_{-1}:x_0x_1 \ldots)
 \= \ldots x_{-1}x_0:x_1 \ldots.\] It is an invertible map with inverse 
 \[ \overline{f}^{-1}(\ldots x_{-2}x_{-1}:x_0x_1 \ldots) \= \ldots x_{-2}:x_{-1}x_0x_1 \ldots.\]
 Note that \[ \pi_0 \circ \overline{f} = f \circ \pi_0. \] So $\overline{f}$ is an extension of $f$.
 Moreover, it is the smallest extension that is invertible, thus, any other invertible extension of $f$ is
 an extension of $\overline{f}$.
 
 If $\overline{\nu}$ is an $\overline{f}-$invariant measure, then $\nu \= \overline{\nu} \circ \pi_0^{-1}$
 is an $f-$invariant measure. We call this $\nu$ the \emph{projection of $\overline{\nu}.$}
 
 On the other hand, if $\nu$ is an $f-$invariant measure, there exists a unique measure $\overline{\nu}$,
 that is $\overline{f}-$invariant, and that for every Borel set $A \subset I$ and for every $n \leq 0$ 
 we have
 \[ \overline{\nu}(\{ \overline{x} \in \hI \colon x_n \in A \}) = \nu(A). \] We call $\overline{\nu}$ 
 the \emph{lift of $\nu$.} It can be proved that in this case \[ \nu = \overline{\nu} \circ \pi_0^{-1}.\]
 So projection and lift of measures are inverse operations. Thus, $f-$invariant measures are in bijection
 with $\overline{f}-$invariant probability measures. Moreover, they preserve the Kolmogorov-Sinai entropy,
 see [Roh61].
 
For $\overline{x} \in \hI$ such that $\pi_k(\overline{x}) \notin \cS$ for every $k \in \Z$, define
\begin{equation}
    D\overline{f}^n(\overline{x}) \= Df^n(\pi_0(\overline{x})),
\end{equation}
 and
 \begin{equation}
 \label{eq:back_derivative}
    D\overline{f}^{-n}(\overline{x}) \= \left[ \displaystyle\prod_{i = 0}^{-n-1} f'(f^i(\pi_{-n}(\overline{x})))
    \right]^{-1},
\end{equation}
for every $n \geq 0$.

For every $\overline{x} \in \overline{I}$ the \emph{forward Lyapunov exponent of $\overline{f}$ at 
$\overline{x}$} as \[ \chi_F(\overline{f},\overline{x}) \= \lim_{n \to \infty} \frac{1}{n} 
\log |D\overline{f}^n(\overline{x})|,\] when the limit exists. In the same way we define the 
\emph{backward Lyapunov exponent of $\overline{f}$ at $\overline{x}$} as
\[\chi_F(\overline{f},\overline{x}) \= \lim_{n \to \infty} \frac{-1}{n} \log
|D\overline{f}^{-n}(\overline{x})|,\] when the limit exist.
By Proposition \ref{prop:2} we have that, for every $\overline{x} \in \overline{PS}$,
$\chi_F(\overline{f}, \overline{x})$ is not well defined.For every $\overline{x} \in \overline{I}$ we put 
\begin{equation}
    \label{eq:upper_ext_B_Lyap_exp}
    \chi_F^+(\overline{f},\overline{x}) \= \limsup_{n \to \infty} \frac{-1}{n} \log
    |D\overline{f}^{-n}(\overline{x})|,
\end{equation}
and
\begin{equation}
    \label{eq:lower_ext_B_Lyap_exp}
    \chi_F^-(\overline{f},\overline{x}) \= \liminf_{n \to \infty} \frac{-1}{n} \log
    |D\overline{f}^{-n}(\overline{x})|.
\end{equation}

Observe, that from \eqref{eq:back_derivative} we have that
\begin{equation}
    \nonumber
    D\overline{f}^{-n}(\overline{x}) = \left[ Df^n(\pi_{-n}(\overline{x})) \right]^{-1}.
\end{equation}
From the above and \eqref{eq:n_derivative} we get
\begin{equation}
    \label{eq:back_n-derivative}
    D\overline{f}^{-n}(\overline{x}) = \lambda^{-n} \frac{h'(h^{-1}(x_{-n}))}{h'(h^{-1}(x_0)))}.
\end{equation}
Then
\begin{equation}
    \label{eq:upper_ext_B_Lyap_exp_2}
    \chi_B^+(\overline{f},\overline{x}) = \log \lambda - \limsup \frac{1}{n} \log |h'(h^{-1}(x_{-n}))|,
\end{equation}
and
\begin{equation}
    \label{eq:lower_ext_B_Lyap_exp_2}
    \chi_B^-(\overline{f},\overline{x}) = \log \lambda - \liminf \frac{1}{n} \log |h'(h^{-1}(x_{-n}))|.
\end{equation}

Let \[ \overline{PS} \= \{ \overline{x} \in \overline{I} \colon \pi_0(\overline{x}) \in 
\overline{\cO_f(h(c))} \}.  \]

\begin{lemm}
\label{lemm:backward_ret_time}
For every $\overline{x} = \ldots x_{-2x_{-1}}\colon x_0 x_1 \ldots$ in $\overline{PS}$ there exists an
increasing sequence of positive integers $\{ n_i \}_{i \geq 1}$ such that
\[ \pi_{-n_i}(\overline{x}) = x_{-n_i} \in h(I_{\hat{k}+i}) \hspace{1cm} \text{and} \hspace{1cm}
\pi_{-m}(\overline{x}) = x_{-m} \notin h(I_{\hat{k} + i}),\] for all $i \geq 1$ and all 
$n_i + 1 \leq m < n_{i+1}. $ Moreover, 
\[ S(\hk + i +1)- S(\hk +1) + t \leq n_i \leq S(\hk + i+2) - S(\hk +2) + t,  \] for all $i \geq 1$. Where
$0 \leq t \leq S(\hk)$.
\end{lemm}

\begin{proof}
 The proof of this lemma follows the same idea of the proof of Lemma \ref{lemm:time_bound}. Let 
 $\overline{x} = \ldots x_{-2x_{-1}}\colon x_0 x_1 \ldots$ in $\overline{PS}$. Recall that for
 every $k \geq 1 $, the sets \[ h(I_k), h(I_k^1), \ldots, h(I_k^{S(k-1) - 1}), h(J_k), h(J_k^1), \ldots, 
 h(J_k^{S(k-2) - 1}),\] are pairwise disjoints and cover $\overline{\cO_f(h(c))}$. Then
 \[ x_0 \in h(I_{\hk}^{t_1}) \hspace{1cm} \text{ or } \hspace{1cm} x_0 \in h(J_{\hk}^{t_2}), \] for some
 $0 \leq t_1 < S(k-1)$ and $0 \leq t_2 < S(k-2).$ Then $f^{t_1}(x_{-t_1}) \in h(I_{\hk}^{t_1})$ or
 $f^{t_2}(x_{-t_2}) \in h(J_{\hk}^{t_2})$. In the former case $x_{-t_1} \in h(I_{\hk})$ so $t = t_1$. In
 the later case $x_{-t_2} \in h(J_{\hk})$, so $f(x_{-(t_2 + 1)}) \in h(J_{\hk})$, 
 thus $x_{-(t_2 + 1)} \in h(I_{\hk}^{S(k-1)-1})$. This implies that 
 $x_{-(t_2 + S(\hk -1))} \in h(I_{\hk})$, so $t = t_2 + S(\hk -1)$. Since $0 \leq t_2 < S(\hk -2)$ we get
 $0 \leq t < S(\hk)$. 
 
 By \eqref{eq:J_k_I_k}  
 \[ x_{-t} \in h(I_{\hk + 1}) \hspace{1cm} \text{ or } \hspace{1cm} x_{-t} \in h(J_{\hk +1}). \] 
 If $x_{-t} \in h(I_{\hk + 1})$ we have that $f(x_{-(t + 1)}) \in h(I_{\hk + 1})$, so
 \[ x_{-(t+1)} \in h(J_{\hk +1}^{S(\hk -1) -1}) \hspace{1cm} \text{ or } \hspace{1cm} x_{-(t+1)} \in 
 h(I_{\hk +1}^{S(\hk) -1}).\]
 In the former case, for every $1 \leq j \leq S(\hk -1)$  
 \[ x _{-(t + j)} \in h(J_{\hk +1})^{S(\hk - 1) -j}. \] From the above 
 \[f(x_{-(t + S(\hk - 1) +1)}) \in h(J_{\hk+1}),\] so 
 $x_{-(t + S(\hk - 1) +1)} \in h(I_{\hk+1}^{S(\hk) -1})$. Then, for every $1 \leq m < S(\hk)$
 \[ x_{-(t + S(\hk - 1) +m)} \in h(I_{\hk+1}^{S(\hk) -m}), \] and
 \[ x_{-(t + S(\hk - 1) + S(\hk))} \in h(I_{\hk+1}). \] In this case $n_1 = t + S(\hk +1)$.
 In the later case, for every $1 \leq j < S(\hk )$  
 \[ x _{-(t + j)} \in h(I_{\hk +1})^{S(\hk) -j}. \] From the above 
 \[x_{-(t + S(\hk))} \in h(I_{\hk+1}).\] In this case $n_1 = t + S(\hk)$.  
 
 If $x_{-t} \in h(J_{\hk + 1})$ we have that $f(x_{-(t + 1)}) \in h(J_{\hk + 1})$, so 
 \[ x_{-(t+1)} \in h(I_{\hk +1}^{S(\hk) -1}). \] This implies that for every $1 \leq m < S(\hk)$
 \[ x_{-(t + m)} \in h(I_{\hk + 1}^{S(\hk - m)}), \] and 
 \[ x_{-(t + S(\hk))} \in h(I_{\hk + 1}). \] In this cas $n_1 = t + S(\hk)$. Thus, we have that 
 \[ S(\hk) + t \leq n_1 \leq S(\hk +1) + t. \]
 
 The construction of the rest of the $n_i$ can be done inductively. Suppose that we have $n_i$ satisfying 
 the conditions in the lemma, thus \[ x_{n_i} \in h(I_{k+i}), \] and 
 \[ S(\hk +i+1) - S(\hk +1) + t \leq n_i \leq S(\hk + i+2) - S(\hk +2) + t. \] Then, by \eqref{eq:J_k_I_k}
 \[ x_{-n_i} \in h(I_{\hk + i+ 1})\hspace{1cm} \text{ or }\hspace{1cm} x_{-n_i} \in h(J_{\hk + + 1}).\]
 If $x_{-n_i} \in h(I_{\hk + i+1})$ we have that $f(x_{-(n_i + 1)}) \in h(I_{\hk +i+ 1})$, so
 \[ x_{-(n_i+1)} \in h(J_{\hk +i+1}^{S(\hk+i -1) -1}) \hspace{1cm} \text{ or } \hspace{1cm} 
 x_{-(n_i+1)} \in h(I_{\hk+i +1}^{S(\hk+i) -1}).\]
 In the former case, for every $1 \leq n \leq S(\hk +i-1)$  
 \[ x _{-(n_i + n)} \in h(J_{\hk +i +1})^{S(\hk +i- 1) -n}. \] From the above 
 \[f(x_{-(n_i + S(\hk+i - 1) +1)}) \in h(J_{\hk+i+1}),\] so 
 $x_{-(n_i + S( \hk+i - 1) +1)} \in h(I_{\hk+i+1}^{S(\hk+i) -1})$. Then, for every $1 \leq m < S(\hk+i)$
 \[ x_{-(n_i + S(\hk+i - 1) +m)} \in h(I_{\hk+i+1}^{S(\hk+i) -m}), \] and
 \[ x_{-(n_i + S(\hk+i - 1) + S(\hk+i))} \in h(I_{\hk+i+1}). \] In this case $n_{i+1} = n_i + S(\hk+i+1)$.
 In the later case, for every $1 \leq n < S(\hk+i)$  
 \[ x _{-(n_i + n)} \in h(I_{\hk+i +1})^{S(\hk) -n}. \] From the above 
 \[x_{-(n_i + S(\hk+i))} \in h(I_{\hk+i+1}).\] In this case $n_{n_i+1} = n_i + S(\hk+i)$. 
 
  If $x_{-n_i} \in h(J_{\hk+i + 1})$ we have that $f(x_{-(n_i + 1)}) \in h(J_{\hk+i + 1})$, so 
 \[ x_{-(n_i+1)} \in h(I_{\hk+i +1}^{S(\hk+i) -1}). \] This implies that for every $1 \leq n < S(\hk+i)$
 \[ x_{-(n_i + n)} \in h(I_{\hk+i + 1}^{S(\hk+i) - m)}), \] and 
 \[ x_{-(n_i + S(\hk+i))} \in h(I_{\hk+i + 1}).\] In this case $n_{i+1}=n_i+S(\hk+i)$. Thus, we have that 
 \[ S(\hk+i+2) - S(\hk+1) + t \leq n_{n_i+1} \leq S(\hk+i+3) - S(\hk+2) + t.\] This conclude the proof.
\end{proof}

\begin{lemm}
\label{lem:back_lyap_exp}
For any $\overline{x} \in \overline{PS}$ such that $x_n \neq h(c)$ for every $n \in \Z$, we have that 
\[ \chi_B^-(\overline{f}, \overline{x}) \leq \log \lambda < (1 + \alpha) \log \lambda 
\leq \chi_B^+(\overline{f}, \overline{x}).\]
\end{lemm}

\begin{proof}
 Let $\overline{x} \in \overline{PS}$ and $\{ n_i\}_{i\geq 1}$ as in Lemma \ref{lemm:backward_ret_time}.
 By \eqref{eq:seq_bound} and \eqref{eq:lower_ext_B_Lyap_exp_2} we have that 
 \[ \chi_B^-(\overline{f},\overline{x}) \leq \log \lambda. \]
 Now by Lemma \ref{lemm:backward_ret_time}
 \[ \frac{-1}{n_i} \geq \frac{-1}{S(\hk + i + 1) - S(\hk +1)}. \] Since $x_{n_i} \in h(I_{\hk + i})$, we
 have $h^{-1}(x_{n_i}) \in I_{\hk + i}$, for all $i \geq 1$. Then, by \eqref{eq:left_crit_point},
 \eqref{eq:right_crit_point}, taking $\alpha \= \max \{ \alpha^+, \alpha^-  \}$
 
 \begin{eqnarray}
      |h'(h^{-1}(x_{-n_i}))| &\leq& e^M|h^{-1}(x_{-n_i})|^{\alpha} \nonumber \nonumber \\
                            &\leq& e^M |D_{\hk + i}|^{\alpha}. \nonumber
 \end{eqnarray}
 Then, letting $N_i \= \frac{-\alpha \log \lambda^{S(\hk + i +1)}|D_{\hk +i}|}{S(\hk + i +1)- S(\hk +1)} 
 - \frac{M}{n_i}$
 \begin{eqnarray}
     \frac{-1}{n_i} \log |h'(h^{-1}(x_{-n_i}))| &\geq& \frac{-1}{S(\hk + i +1)- S(\hk +1)} 
    \log |D_{\hk +i}|^{\alpha} - \frac{M}{n_i} \nonumber \\
                                                &=& \frac{-1}{S(\hk + i +1)- S(\hk +1)} 
    \left[ - \alpha S(\hk + i +1) \log \lambda \right] + N_i. \nonumber
 \end{eqnarray}
 Taking limit as $i \to \infty$ we get
 \[\lim_{i \to \infty}  \frac{-1}{n_i} \log |h'(h^{-1}(x_{-n_i}))| \geq \alpha \log \lambda. \]
 So we have
 \[ \chi_B^-(\overline{f},\overline{x}) \leq \log \lambda < (1 + \alpha)\log \lambda
  \leq \chi_B^+(\overline{f}, \overline{x}).\]
\end{proof}

% %%% Local Variables:
% %%% mode: latex
% %%% TeX-master: "Unbounded_Lyapunov_exponent"
%%% End:
